# Supplementary material for: MedGame: Storytelling Gamification Empowered by Large Language Models for Medical Education
Source: arXiv:2607.21570 source file (2026-11-25)
Supplement: Supplementary file 1 [file clinical_story_tikz.tex]

\documentclass[tikz,border=10pt]{standalone}
\usepackage[utf8]{inputenc}
\usepackage[T1]{fontenc}
\usepackage{helvet}

\usetikzlibrary{shapes, arrows.meta, positioning, shadows.blur, calc, fit, backgrounds}

\definecolor{colLevel0}{RGB}{52, 73, 94}
\definecolor{colLevel1}{RGB}{41, 128, 185}
\definecolor{colLevel2}{RGB}{22, 160, 133}
\definecolor{colLevel3}{RGB}{230, 126, 34}
\definecolor{colLevel4}{RGB}{142, 68, 173}
\definecolor{colNote}{RGB}{100, 100, 100}
\definecolor{bgGray}{RGB}{245, 245, 245}

\begin{document}

\begin{tikzpicture}[
    node distance=1.8cm and 2.5cm,
    base/.style={
        draw=none,
        rounded corners=4pt,
        align=center,
        blur shadow={shadow blur steps=5, shadow xshift=1pt, shadow yshift=-1pt},
        font=\bfseries\small,
        text=white,
        inner sep=8pt
    },
    level0/.style={base, fill=colLevel0, minimum width=4cm, minimum height=1.2cm},
    level1/.style={base, fill=colLevel1, minimum width=3.5cm, minimum height=1.0cm},
    level2/.style={base, fill=colLevel2, minimum width=3.5cm, minimum height=1.0cm},
    level3/.style={base, fill=colLevel3, minimum width=2.8cm, minimum height=1.0cm, font=\bfseries\footnotesize},
    level4/.style={base, fill=colLevel4, minimum width=3.5cm, minimum height=1.0cm, font=\bfseries\footnotesize},
    note/.style={
        font=\scriptsize\color{darkgray},
        align=left,
        anchor=west
    },
    subtitle/.style={
        font=\footnotesize\color{colNote},
        align=center
    },
    line/.style={
        draw=gray!50,
        -Latex,
        line width=1.2pt,
        rounded corners=10pt
    },
    line_label/.style={
        midway,
        fill=white,
        text=gray,
        font=\tiny,
        inner sep=1pt
    }
]

    \def\levelLabelX{-4.5}

    \def\yLevelZero{0}
    \def\yLevelOne{-2}
    \def\yLevelTwo{-4}
    \def\yLevelThree{-6.5}
    \def\yLevelFour{-10}

    \node[level0] (root) at (0, \yLevelZero) {Clinical\_Story\_Tree};
    \node[note, right=0.3cm of root] (note0) {$\bullet$ target\_students\\$\bullet$ acts[ ]};

    \node[level1] (act) at (0, \yLevelOne) {Act};
    \node[note, right=0.3cm of act] (note1) {$\bullet$ id, title, intro\\$\bullet$ list\_of\_scene[ ]};

    \node[level2] (scene) at (0, \yLevelTwo) {Scene};
    \node[note, right=0.3cm of scene] (note2) {$\bullet$ id, title\\$\bullet$ start/end\_role\_play\\$\bullet$ scene\_item[ ]};

    \node[level3] (batch) at (0, \yLevelThree) {Batch};
    \node[level3] (single) at (-3.5, \yLevelThree) {Single\_Choice};
    \node[level3] (inter) at (3.5, \yLevelThree) {Interactive};

    \node[subtitle, below=0.15cm of single] {Single-answer MCQ};
    \node[subtitle, below=0.15cm of batch] {Multi-select (Panel)};
    \node[subtitle, below=0.15cm of inter] {Info Gathering};

    \node[note, below=0.6cm of single, anchor=north] (note3a) {$\bullet$ question};
    \node[note, below=0.6cm of batch, anchor=north, align=center] (note3b) {$\bullet$ question\\$\bullet$ overall\_explanation\\$\bullet$ submit\_button\_text};
    \node[note, below=0.6cm of inter, anchor=north] (note3c) {$\bullet$ question};

    \node[level4] (std_opt) at (-2, \yLevelFour) {StandardOption};
    \node[note, below=0.15cm of std_opt, align=center, anchor=north] (note4a) {$\bullet$ content, is\_correct\\$\bullet$ explanation, teaching\_point};

    \node[level4] (int_opt) at (3.5, \yLevelFour) {InteractiveOption};
    \node[note, below=0.15cm of int_opt, align=center, anchor=north] (note4b) {$\bullet$ content, is\_correct\\$\bullet$ interaction, type\\$\bullet$ teaching\_point};

    \begin{scope}[on background layer]
        \draw[line] (root) -- (act);

        \draw[line] (act) -- (scene);

        \draw[line] (scene.south) -- ++(0,-0.5) -| (single.north);
        \draw[line] (scene.south) -- (batch.north);
        \draw[line] (scene.south) -- ++(0,-0.5) -| (inter.north);

        \draw[line] (single.south) -- ++(0,-1.2) -| (std_opt.north);
        \draw[line] (batch.south) -- ++(0,-1.8) -| (std_opt.north);
        \draw[line] (inter.south) -- ++(0,-1.2) -- (int_opt.north);
    \end{scope}

\end{tikzpicture}
\end{document}
